# Supplementary material for: Tempering stochastic density functional theory
Source: arXiv:2107.06218 source file (2021-10-16)
Supplement: Supplementary file 1 [file SI_v11.pdf]

# Supporting information for “Tempering embedding stochastic density functional theory”

Minh Nguyen<sup>1</sup>, Wenfei Li<sup>1</sup>, Yangtao Li<sup>1</sup>, Roi Baer<sup>2</sup>, Eran Rabani<sup>3</sup>, Daniel Neuhauser<sup>1</sup>

<sup>1</sup> *Department of Chemistry, University of California at Los Angeles, Los Angeles, California 90095, USA*

<sup>2</sup> *Fritz Haber Center of Molecular Dynamics and Institute of Chemistry, The Hebrew University of Jerusalem, Jerusalem, 91904 Israel*

<sup>3</sup> *Department of Chemistry, University of California and Material Science Division, Lawrence Berkeley National Laboratory, Berkeley, California 94720, USA and Tel Aviv University, Tel Aviv 69978, Israel*

## Polynomial Fit

We use a 2nd order polynomial fit of the form  $g(x) = ax^2 + bx + c$  (where  $x \equiv \beta/\beta^w$ ) of the energies and forces in Figs. 2 and 3 and of their respective errors.

Table SI. 2nd order polynomial fit parameters of the energies values in Fig. 2 in the main text.

| system                             | a        | b        | c       |
|------------------------------------|----------|----------|---------|
| Si <sub>35</sub> H <sub>36</sub>   | 0.006227 | -0.10948 | -24.199 |
| Si <sub>87</sub> H <sub>76</sub>   | 0.004672 | -0.08605 | -24.583 |
| Si <sub>353</sub> H <sub>196</sub> | 0.002147 | -0.04640 | -25.347 |

Table SII. 2nd order polynomial fit parameters of the error in energies values in Fig. 2 in the main text.

| system                             | a         | b         | c       |
|------------------------------------|-----------|-----------|---------|
| Si <sub>35</sub> H <sub>36</sub>   | 0.0006584 | -0.008834 | 0.04004 |
| Si <sub>87</sub> H <sub>76</sub>   | 0.0001339 | -0.004178 | 0.03589 |
| Si <sub>353</sub> H <sub>196</sub> | 0.0000935 | -0.002163 | 0.01570 |

Table SIII. 2nd order polynomial fit parameters of the  $\sigma_F$  values in Fig. 3 in the main text.

| system                             | a         | b         | c       |
|------------------------------------|-----------|-----------|---------|
| Si <sub>35</sub> H <sub>36</sub>   | 0.0003149 | -0.003277 | 0.03334 |
| Si <sub>87</sub> H <sub>76</sub>   | 0.0002627 | -0.003830 | 0.03540 |
| Si <sub>353</sub> H <sub>196</sub> | 0.0002537 | -0.004067 | 0.03389 |

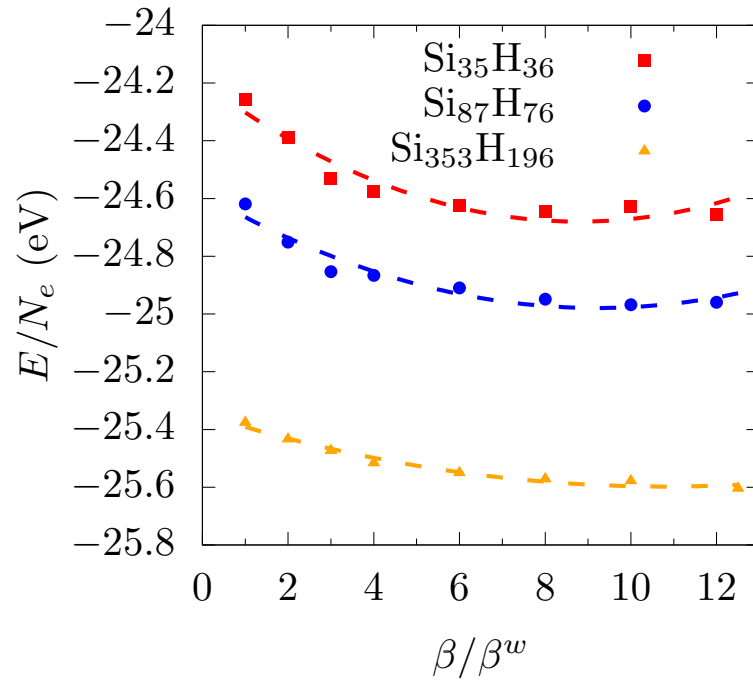

Figure S1: The average energy per electron from Fig. 2 in the main text, with a 2nd order polynomial fit. The parameters of the fit are in Table SI.

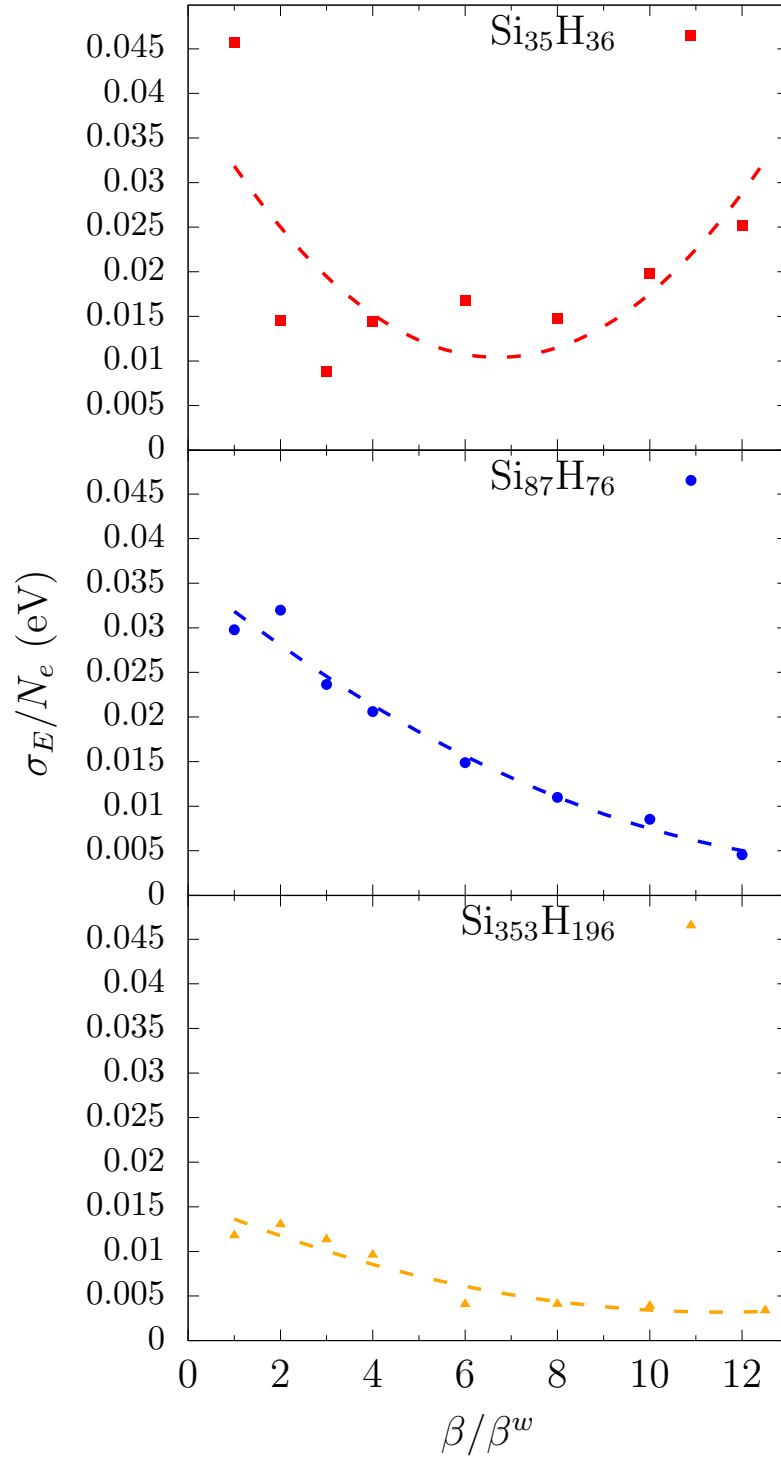

Figure S2: The error-bars from Fig. 2 in the main text and a 2nd order polynomial fit. The parameters of the fit are in Table SII. The error bars are themselves very fluctuating for the smallest system, but due to self-averaging they are much smoother for the larger two systems.

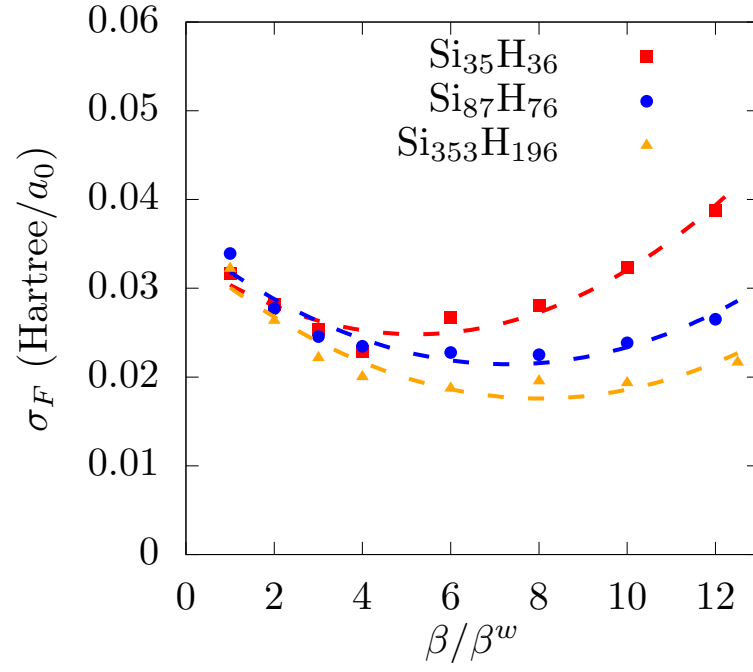

Figure S3: The standard force error  $\sigma_F$  from Fig. 3 in the main text, together with a 2nd order polynomial fit. The parameters of the fit are in Table SIII.
